# Supplementary material for: ComposeAnyone: Controllable Layout-to-Human Generation with Decoupled Multimodal Conditions
Source: arXiv:2501.12173 source file (2025-01-21)
Supplement: Supplementary file 1 [file X_suppl.tex]

\clearpage
\setcounter{page}{1}
\maketitlesupplementary

\section{Additional Implementation Details}
\noindent \textbf{Fine-grained Prompt.} In \Cref{fig:text1}, we illustrate the generation of customized, fine-grained textual inquiries, specifically tailored to distinct attributes across various aspects such as the face, top, bottom, dress, and shoes. These inquiries comprehensively encapsulate the detailed features of each component. The results demonstrate that CogVLM2 successfully generates correctly formatted textual descriptions for approximately 70–80\% of the inquiries. However, certain outputs may fail, yielding responses containing the placeholder keyword "etc." To mitigate this limitation, we either regenerate or filter the outputs based on their corresponding IDs to enhance text accuracy. Furthermore, to ensure the generated text aligns closely with natural human language patterns, we reorganize the string outputs from CogVLM2 to produce the final results.

\section{Additional Experimental Results}
\noindent \textbf{More visual results.}
In \Cref{fig:visual0} and \Cref{fig:visual00}, we showcase additional visual examples of human image generation guided by hand-drawn layouts within a multi-modal input framework. These results further highlight the efficacy of ComposeAnyone in handling decoupled multi-modal inputs, enabling the generation of realistic and high-quality human images. The generated outputs exhibit precise alignment with the spatial configuration of the hand-drawn layouts, faithfully adhere to the intricate details specified in the textual descriptions, and accurately encapsulate the distinctive features of the reference images.

\noindent \textbf{More Qualitative Comparisons.}
In \Cref{fig:visual1}, we provide an extensive quantitative comparison on the DressCode~\cite{morelli2022dresscode} dataset against subject-driven methods. To ensure a more equitable evaluation, we employ a "try-on" paradigm for AnyDoor~\cite{chen2023anydoor} and IP-Adapter~\cite{ye2023ip-adapter}, wherein a specified garment serves as the reference image, and predefined regions of the human image are masked. In contrast, ComposeAnyone generates images guided by the spatial arrangement of a hand-drawn layout, utilizing all human components as reference inputs. This experimental setup is consistently applied in \Cref{fig:comparison1} of the main paper. Notably, despite the heightened complexity of ComposeAnyone's generation task, it surpasses competing baselines in accurately capturing the features of the reference image.
In \Cref{fig:visual2}, we conduct further quantitative comparisons on the VITON-HD~\cite{choi2021vitonhd} dataset against layout-guided text-to-image methods. As the human images in the VITON-HD dataset predominantly depict the upper body, our evaluation focuses on text-conditioned generation for the facial region and upper garments. A similar configuration is adopted in \Cref{fig:comparison2} of the main paper. The results underscore that our approach achieves superior alignment with the spatial arrangement of the hand-drawn layout and the semantic details of text descriptions, while simultaneously producing sharp facial features and photorealistic human images.

\section{User Study}
\begin{figure}[t]
  \centering
  % \fbox{\rule{0pt}{2in} \rule{0.9\linewidth}{0pt}}
   \includegraphics[width=\linewidth]{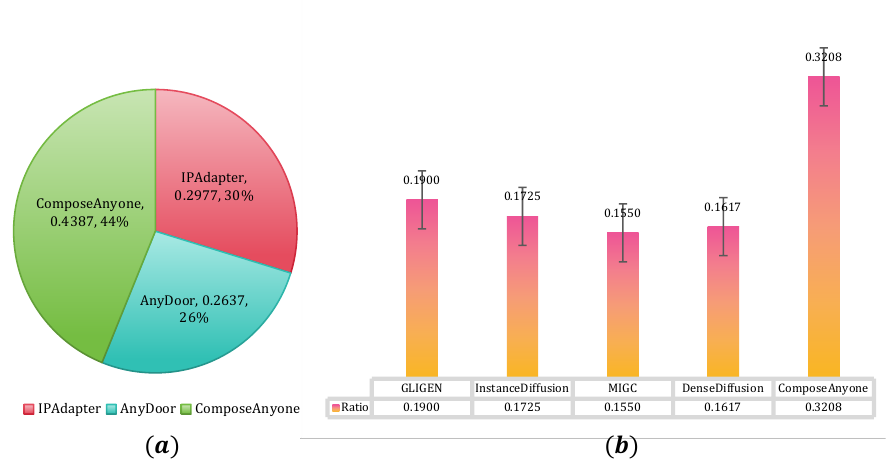}
    % \vspace{-1mm}
   \caption{$(a)$User study results with subject-driven methods.
   $(b)$User study results with layout-guided text-to-image methods.}
   \label{fig:user1}
   % \vspace{-4mm}
\end{figure}

\begin{table}[t]
    \centering
    % \vspace{-1mm}
    \resizebox{0.48\textwidth}{!}{
    % \fontsize{9}{10} \selectfont
    \setlength{\tabcolsep}{1mm}
    \begin{tabular}{l|ccc|c}
        \toprule
        % \multirow{3}{*}{Methods} & \multicolumn{6}{c|}{VITON-HD} & \multicolumn{6}{c}{DressCode} \\
        % \cline{2-13}
        \multirow{2}{*}{Evaluation} & \multicolumn{3}{c|}{Alignment} & \multicolumn{1}{c}{Image Quality} \\
        \cline{2-5}
        & Text & Reference & Layout & -\\
        \midrule
        Score(1—5) & 3.876 & 3.778 & 3.772& 3.747\\

        \bottomrule
    \end{tabular}
    }
    \caption{The user study results on the visual outcomes generated from multimodal conditional inputs.}
    \label{tab:user2}
    \vspace{-1mm}
\end{table}
We conducted a user study with 222 participants spanning diverse identities and age groups to rigorously benchmark our proposed method against established baselines. 
We evaluated ComposeAnyone against layout-guided~\cite{li2023gligen,wang2024instancediffusion,zhou2024migc,densediffusion} and subject-driven approaches~\cite{ye2023ip-adapter,chen2023anydoor}, emphasizing input alignment and image quality through 35 comparative questions. 
As illustrated in \Cref{fig:user1}, our method emerged as the preferred choice for the majority.
Additionally, we assessed ComposeAnyone under multimodal mixed conditions by using 10 evaluation questions. Participants rated its performance on a five-point scale across textual, reference-image, and hand-drawn layout alignment, as well as image quality. The results shown in \Cref{tab:user2} reveal superior alignment across modalities and high-quality, realistic image generation.

\begin{figure*}
  \centering
  \includegraphics[width=\textwidth]{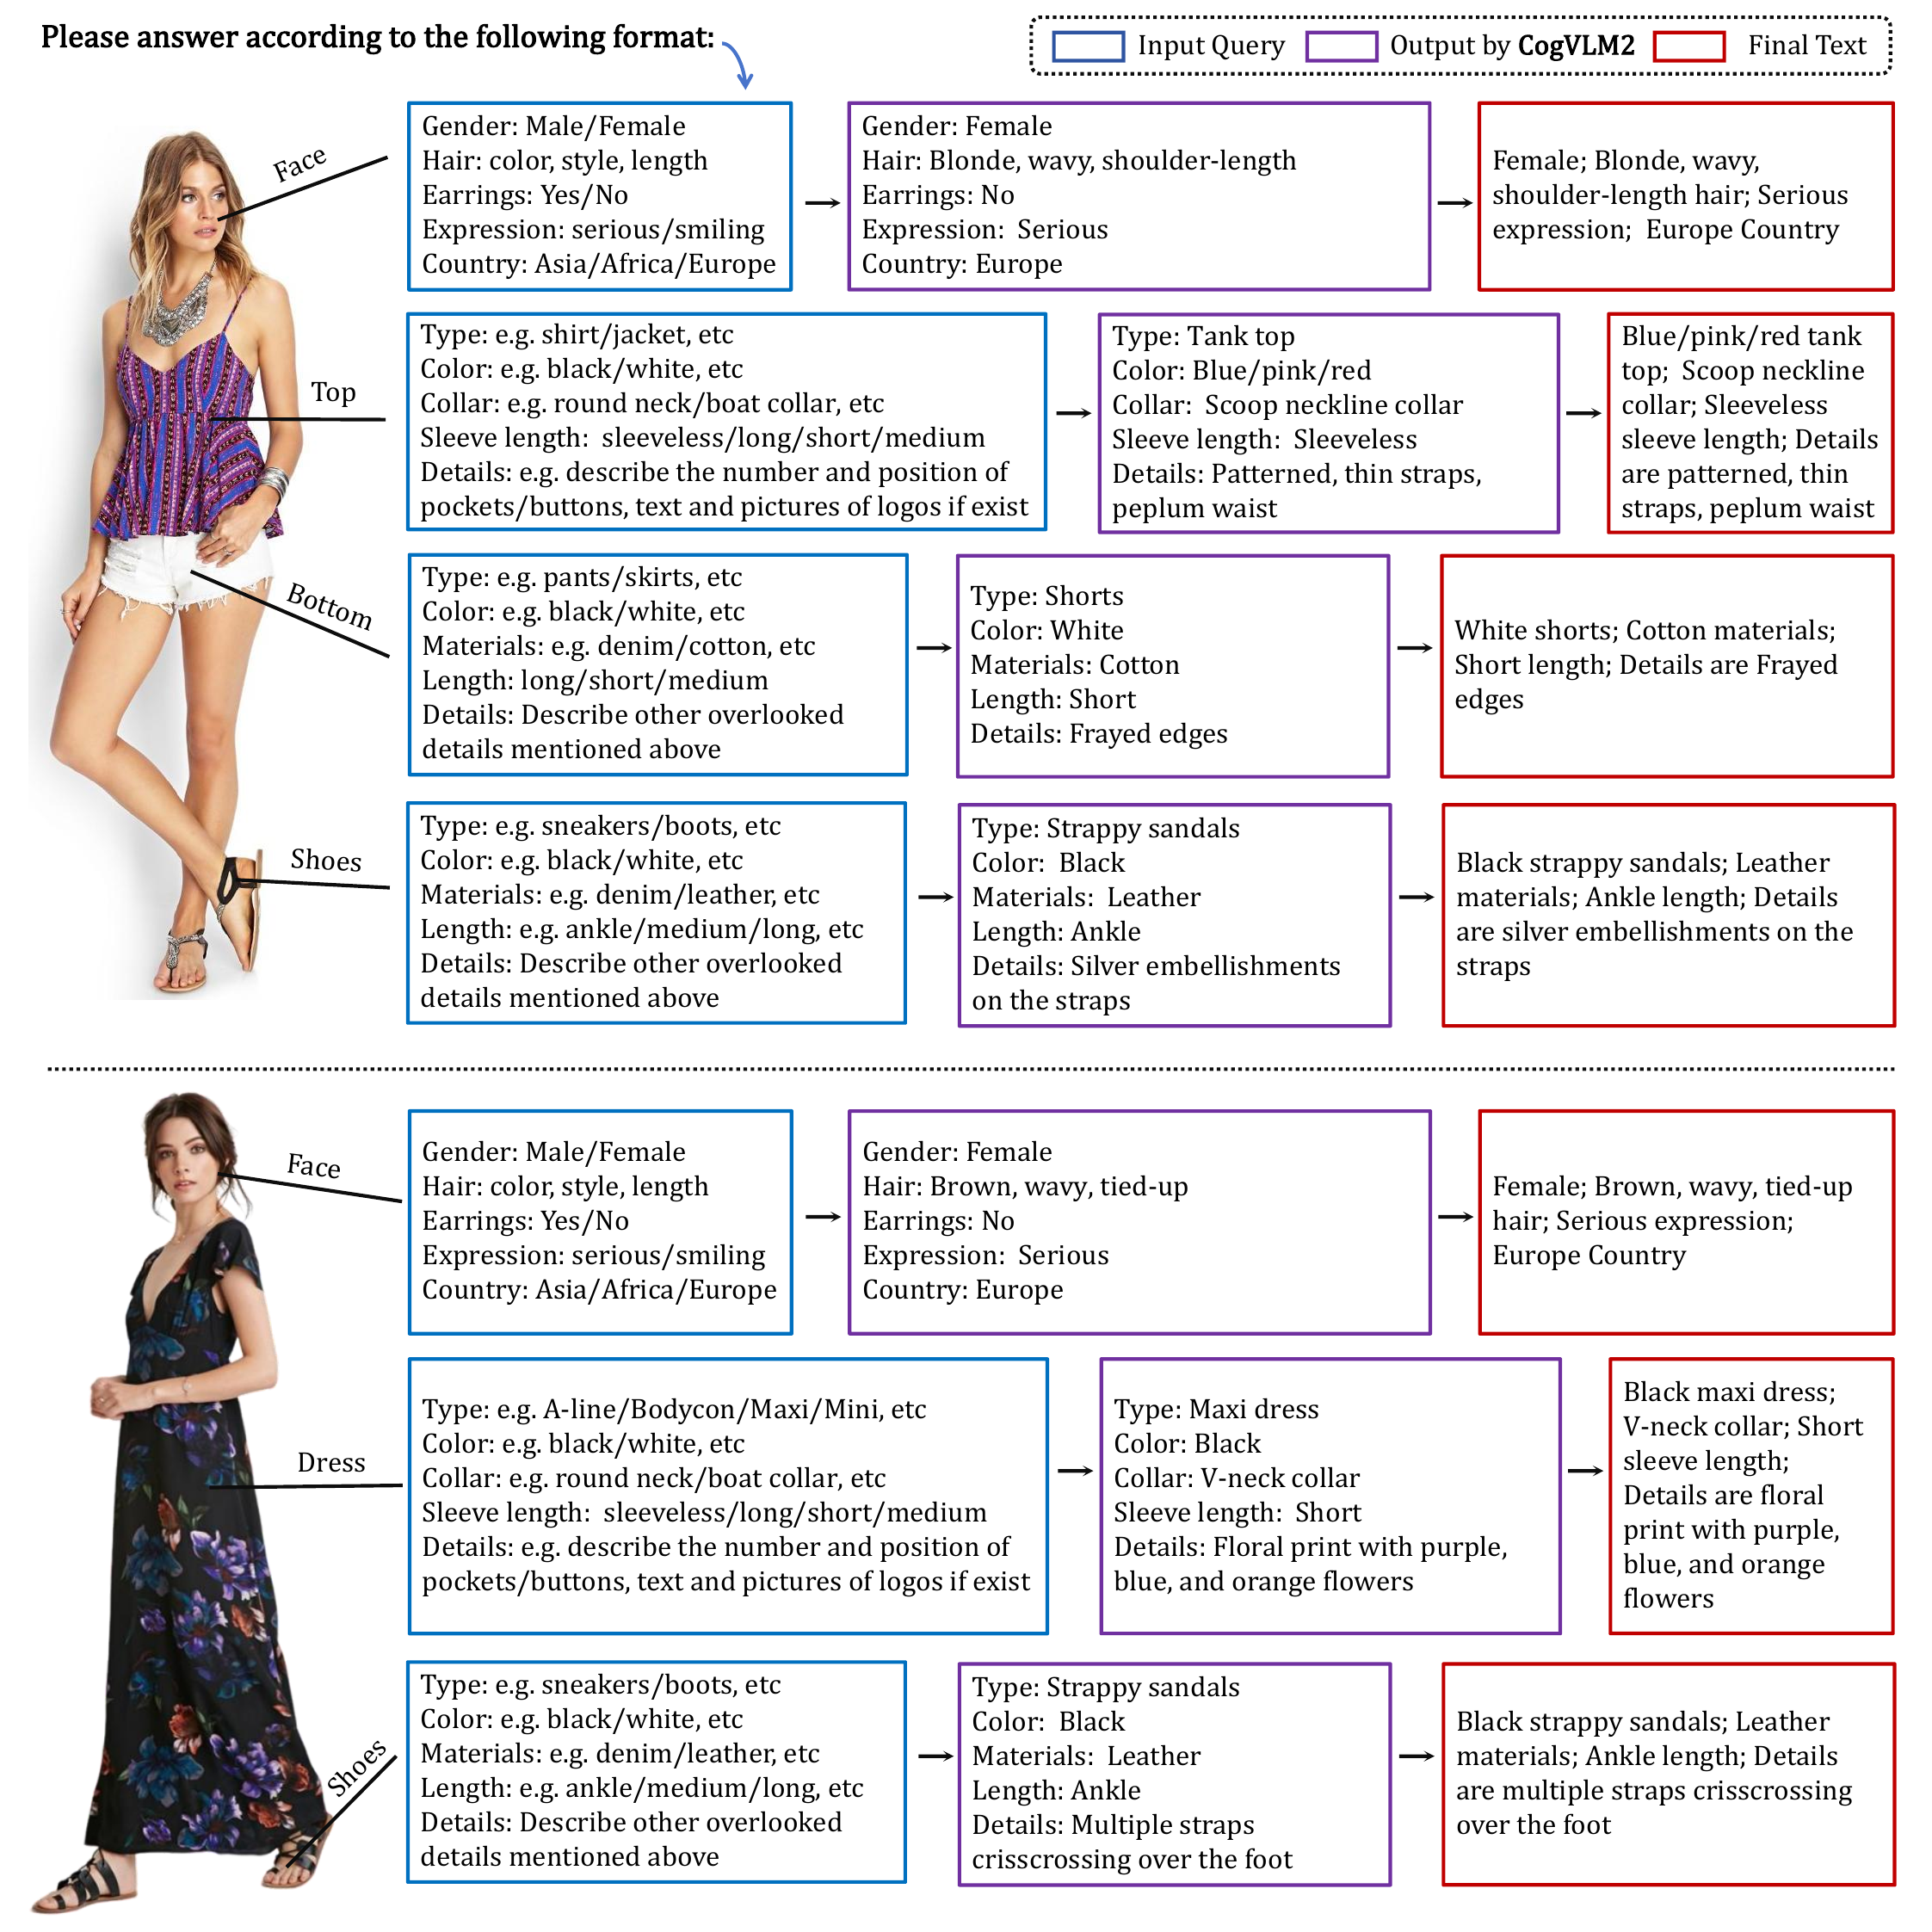}
  % \vspace{-2mm}
  \caption{The fine-grained text descriptions of each component of human image. We use CogVLM2 to extract various attributes corresponding to components. Finally, these attributes are combined and transformed into a single descriptive sentence.
  }
  % \vspace{-2mm}
  \label{fig:text1}
\end{figure*}

\begin{figure*}
  \centering
  \includegraphics[width=0.92\textwidth]{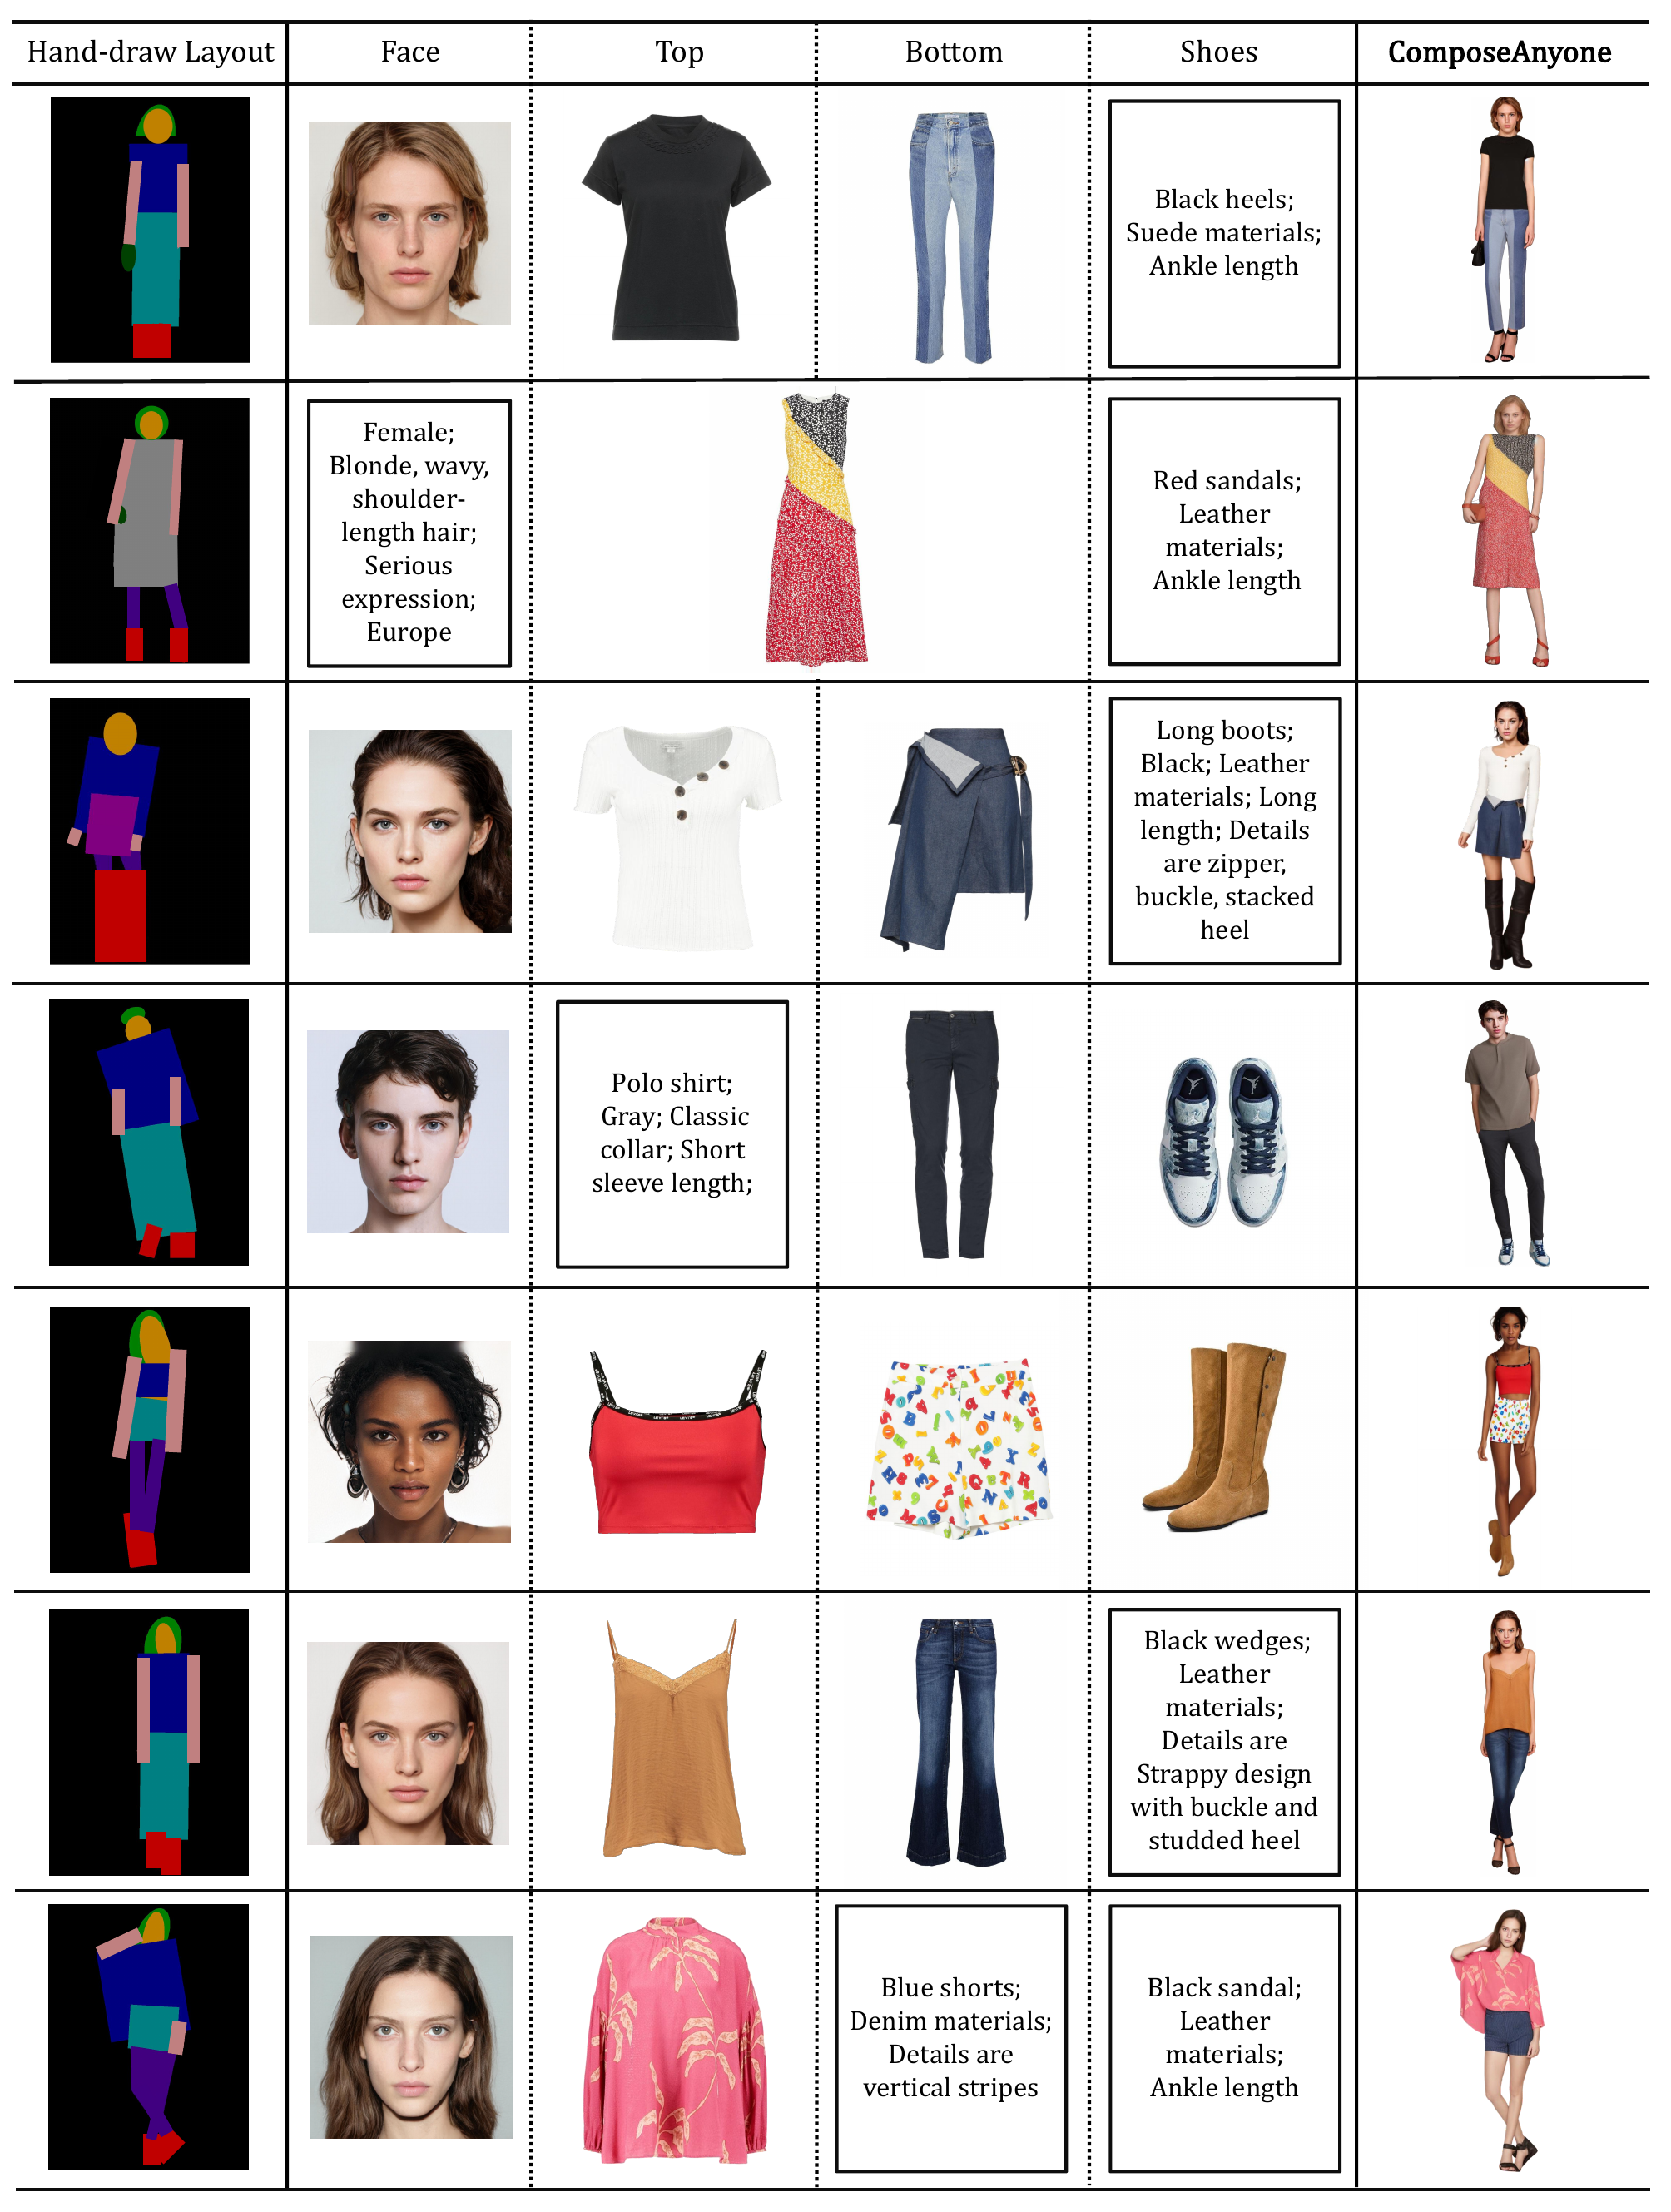}
  % \vspace{-2mm}
  \caption{More visual results of ComposeAnyone, highlighting its ability to process diverse modalities and generate high-quality human images that align with each input.
  }
  % \vspace{-2mm}
  \label{fig:visual0}
\end{figure*}

\begin{figure*}
  \centering
  \includegraphics[width=0.92\textwidth]{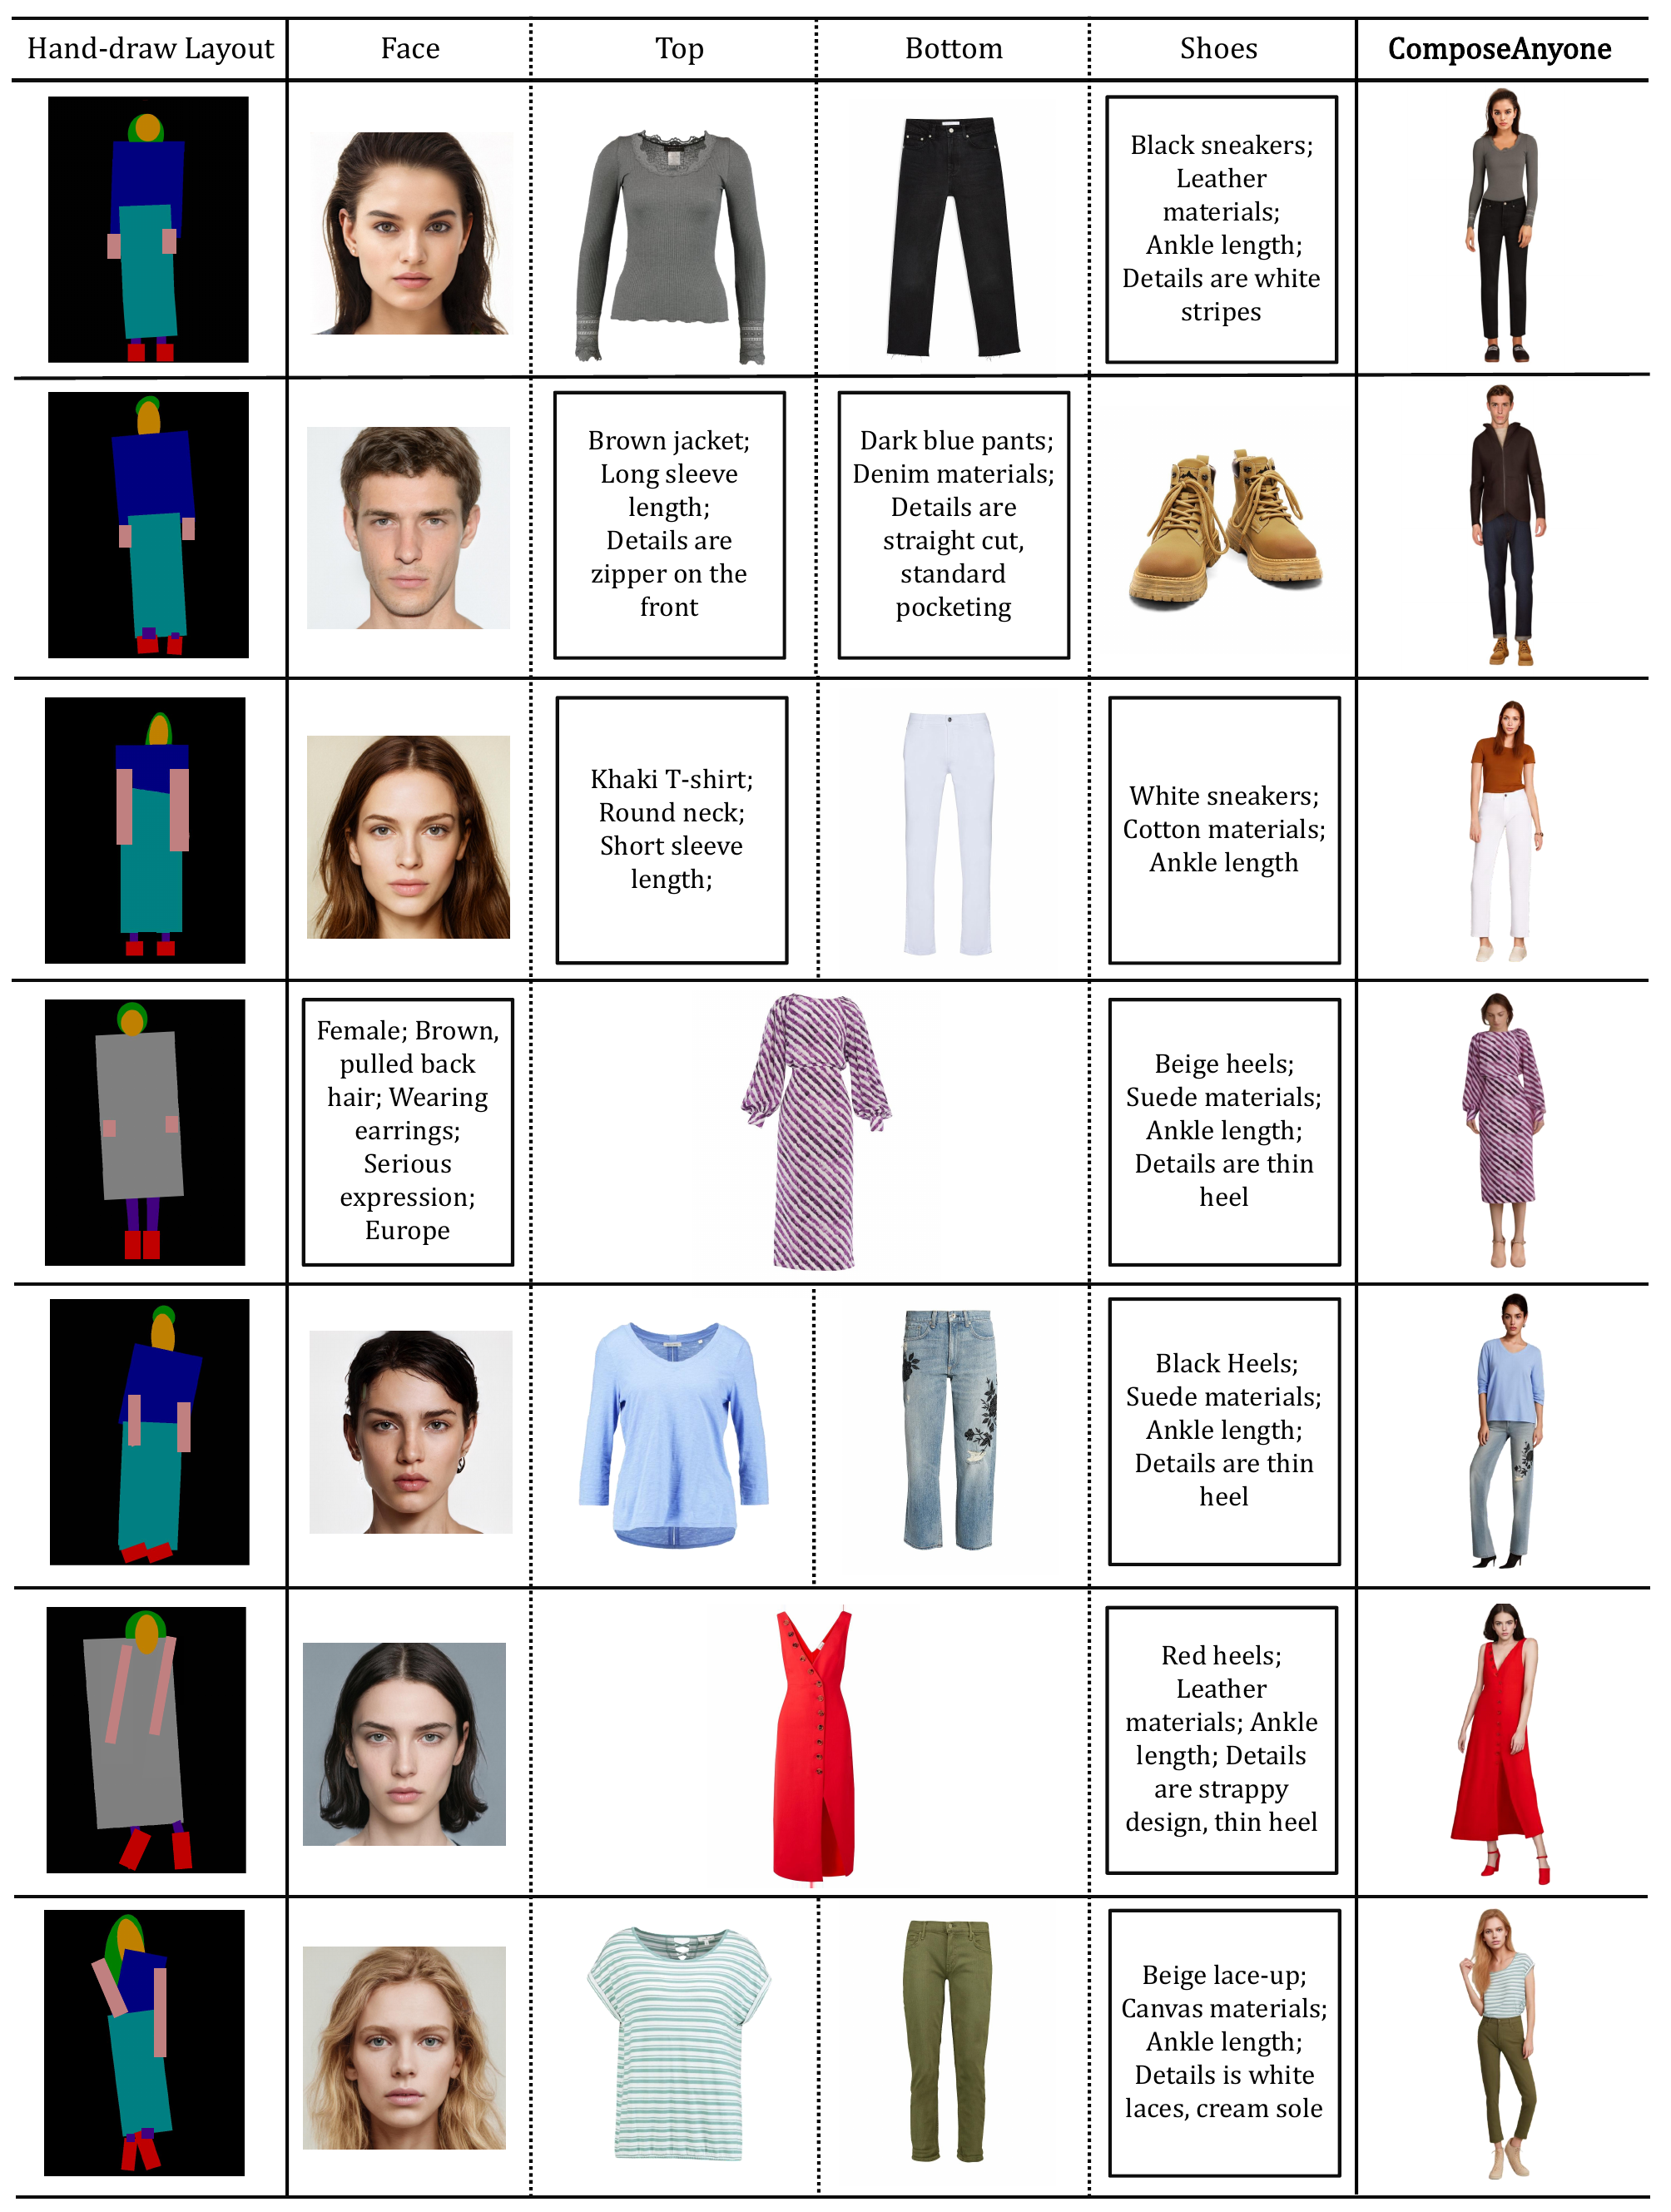}
  % \vspace{-2mm}
  \caption{More visual results of ComposeAnyone, highlighting its ability to process diverse modalities and generate high-quality human
images that align with each input.
  }
  % \vspace{-2mm}
  \label{fig:visual00}
\end{figure*}

\begin{figure*}
  \centering
  \includegraphics[width=\textwidth]{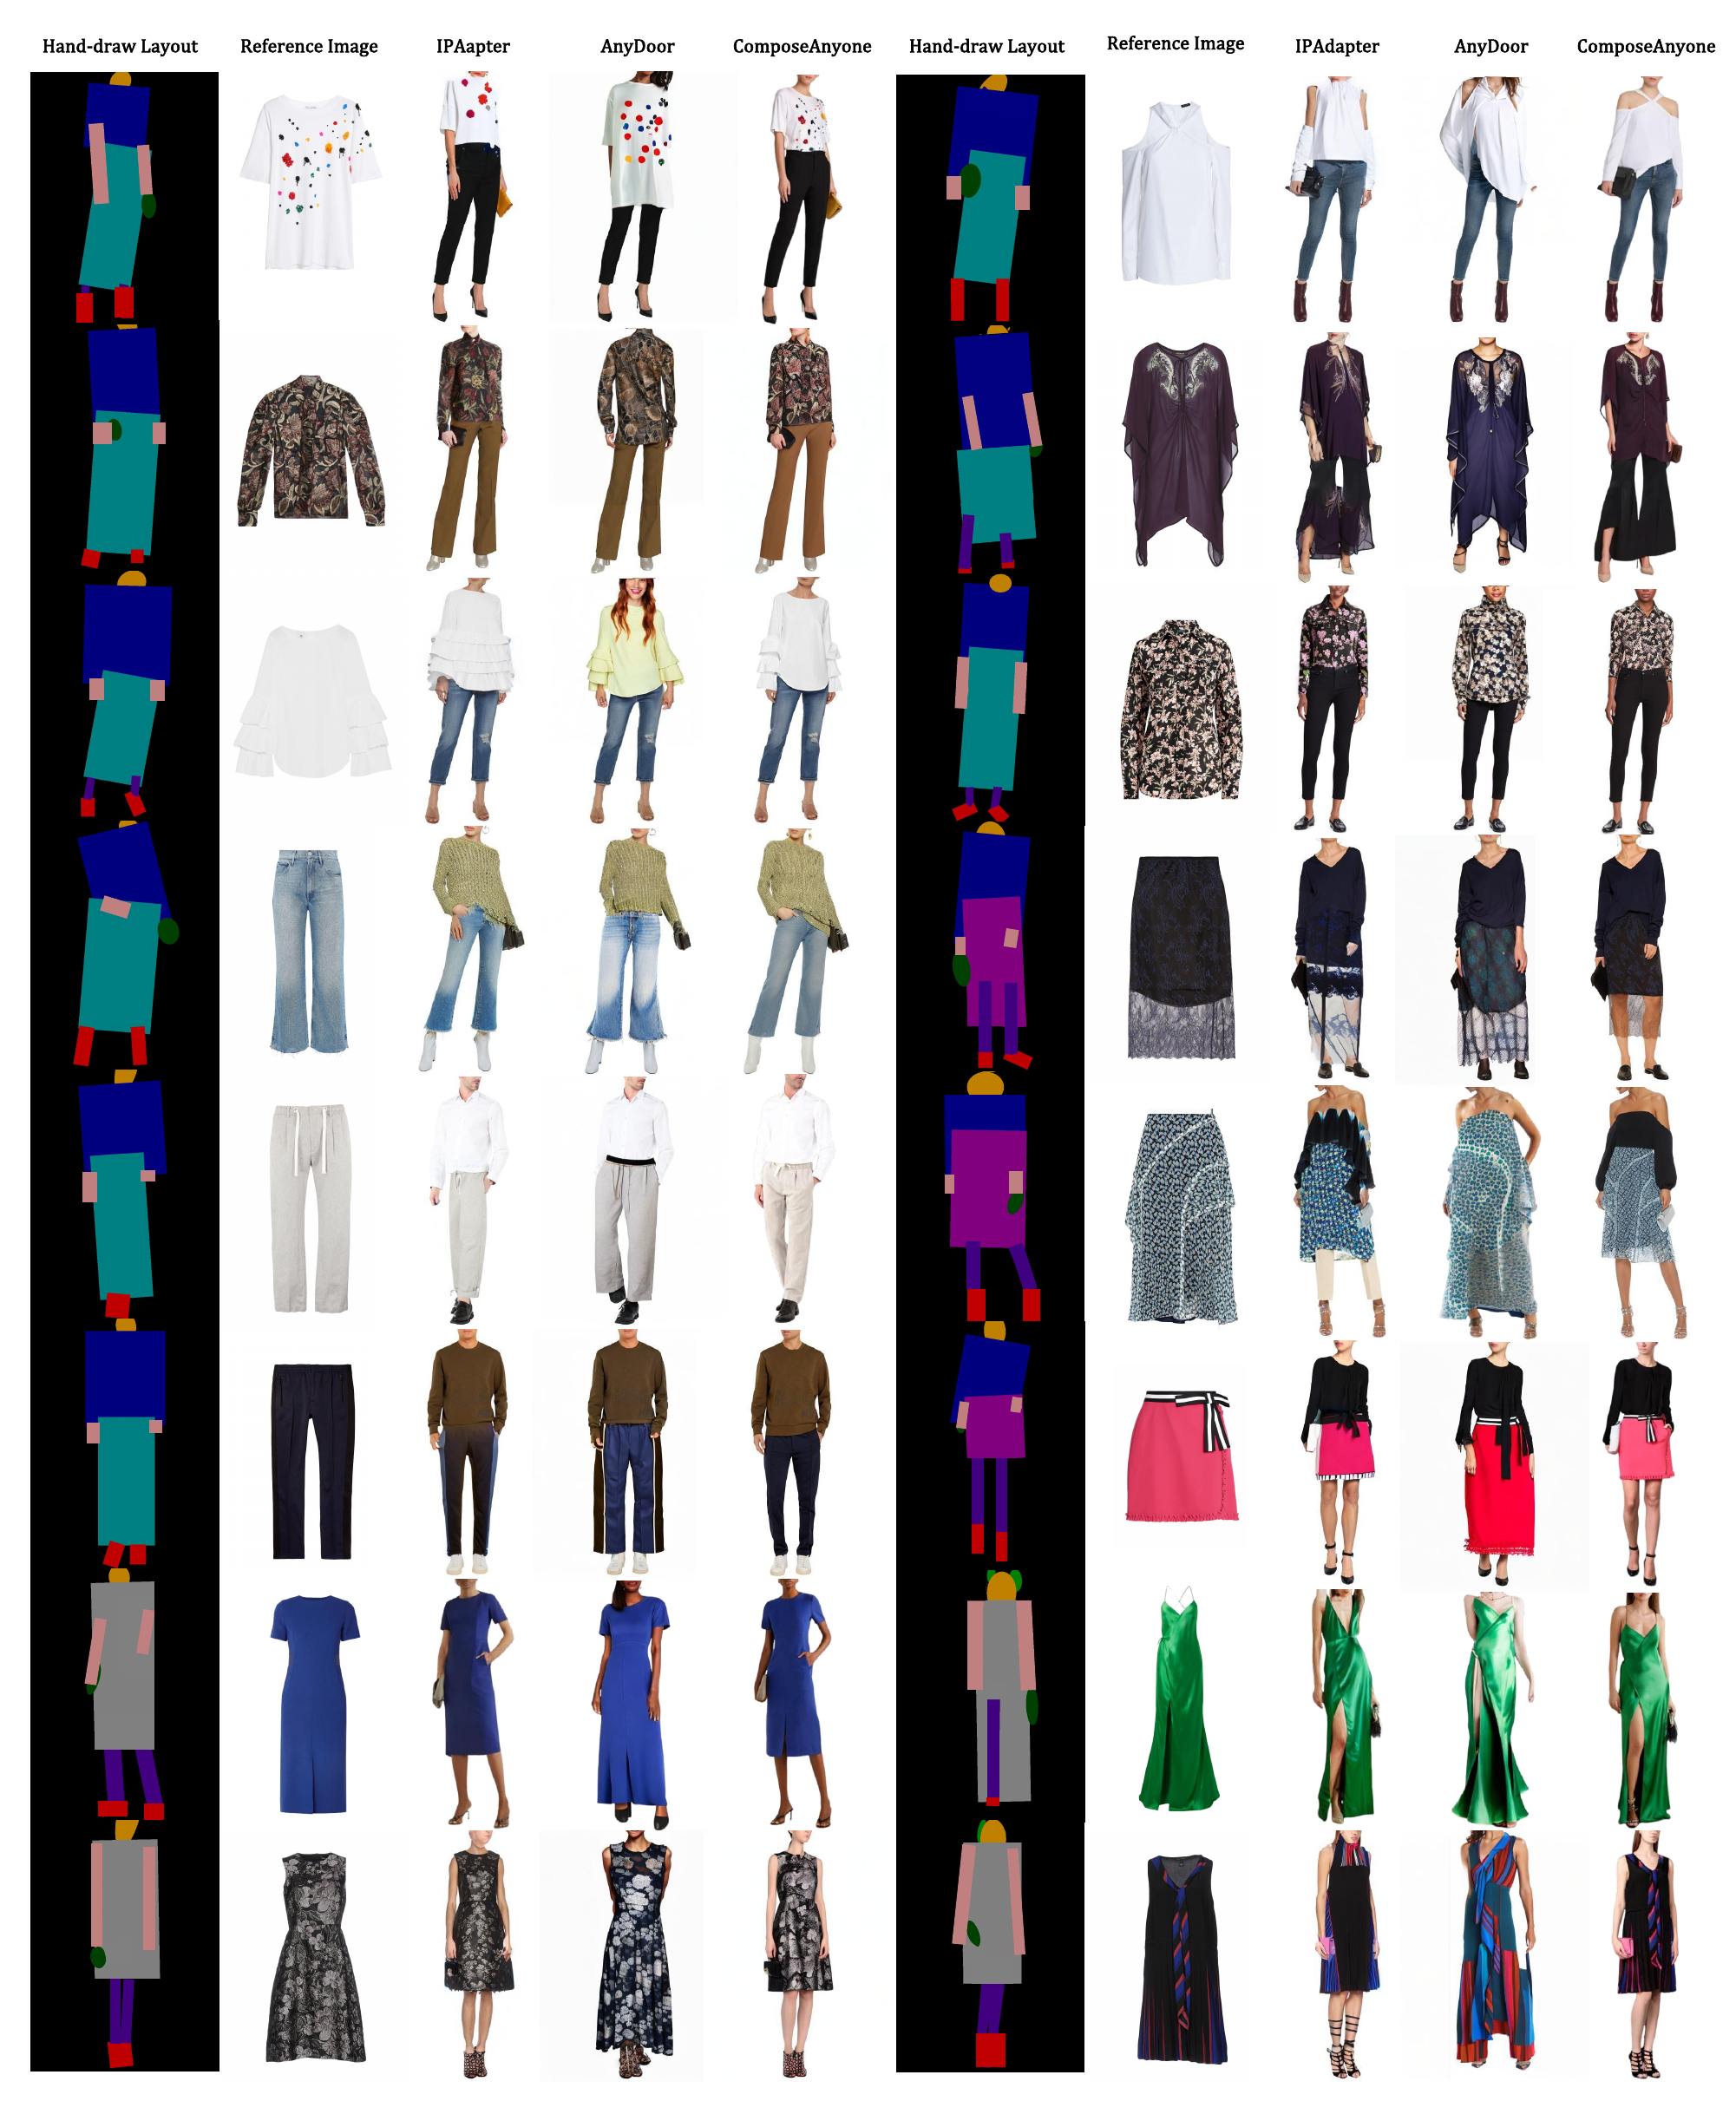}
  % \vspace{-2mm}
  \caption{More qualitative comparison with subject-driven methods on the DressCode dataset. ComposeAnyone demonstrates high fidelity in matching specific features of a given reference cloth image.
  }
  % \vspace{-2mm}
  \label{fig:visual1}
\end{figure*}

\begin{figure*}
  \centering
  \includegraphics[width=\textwidth]{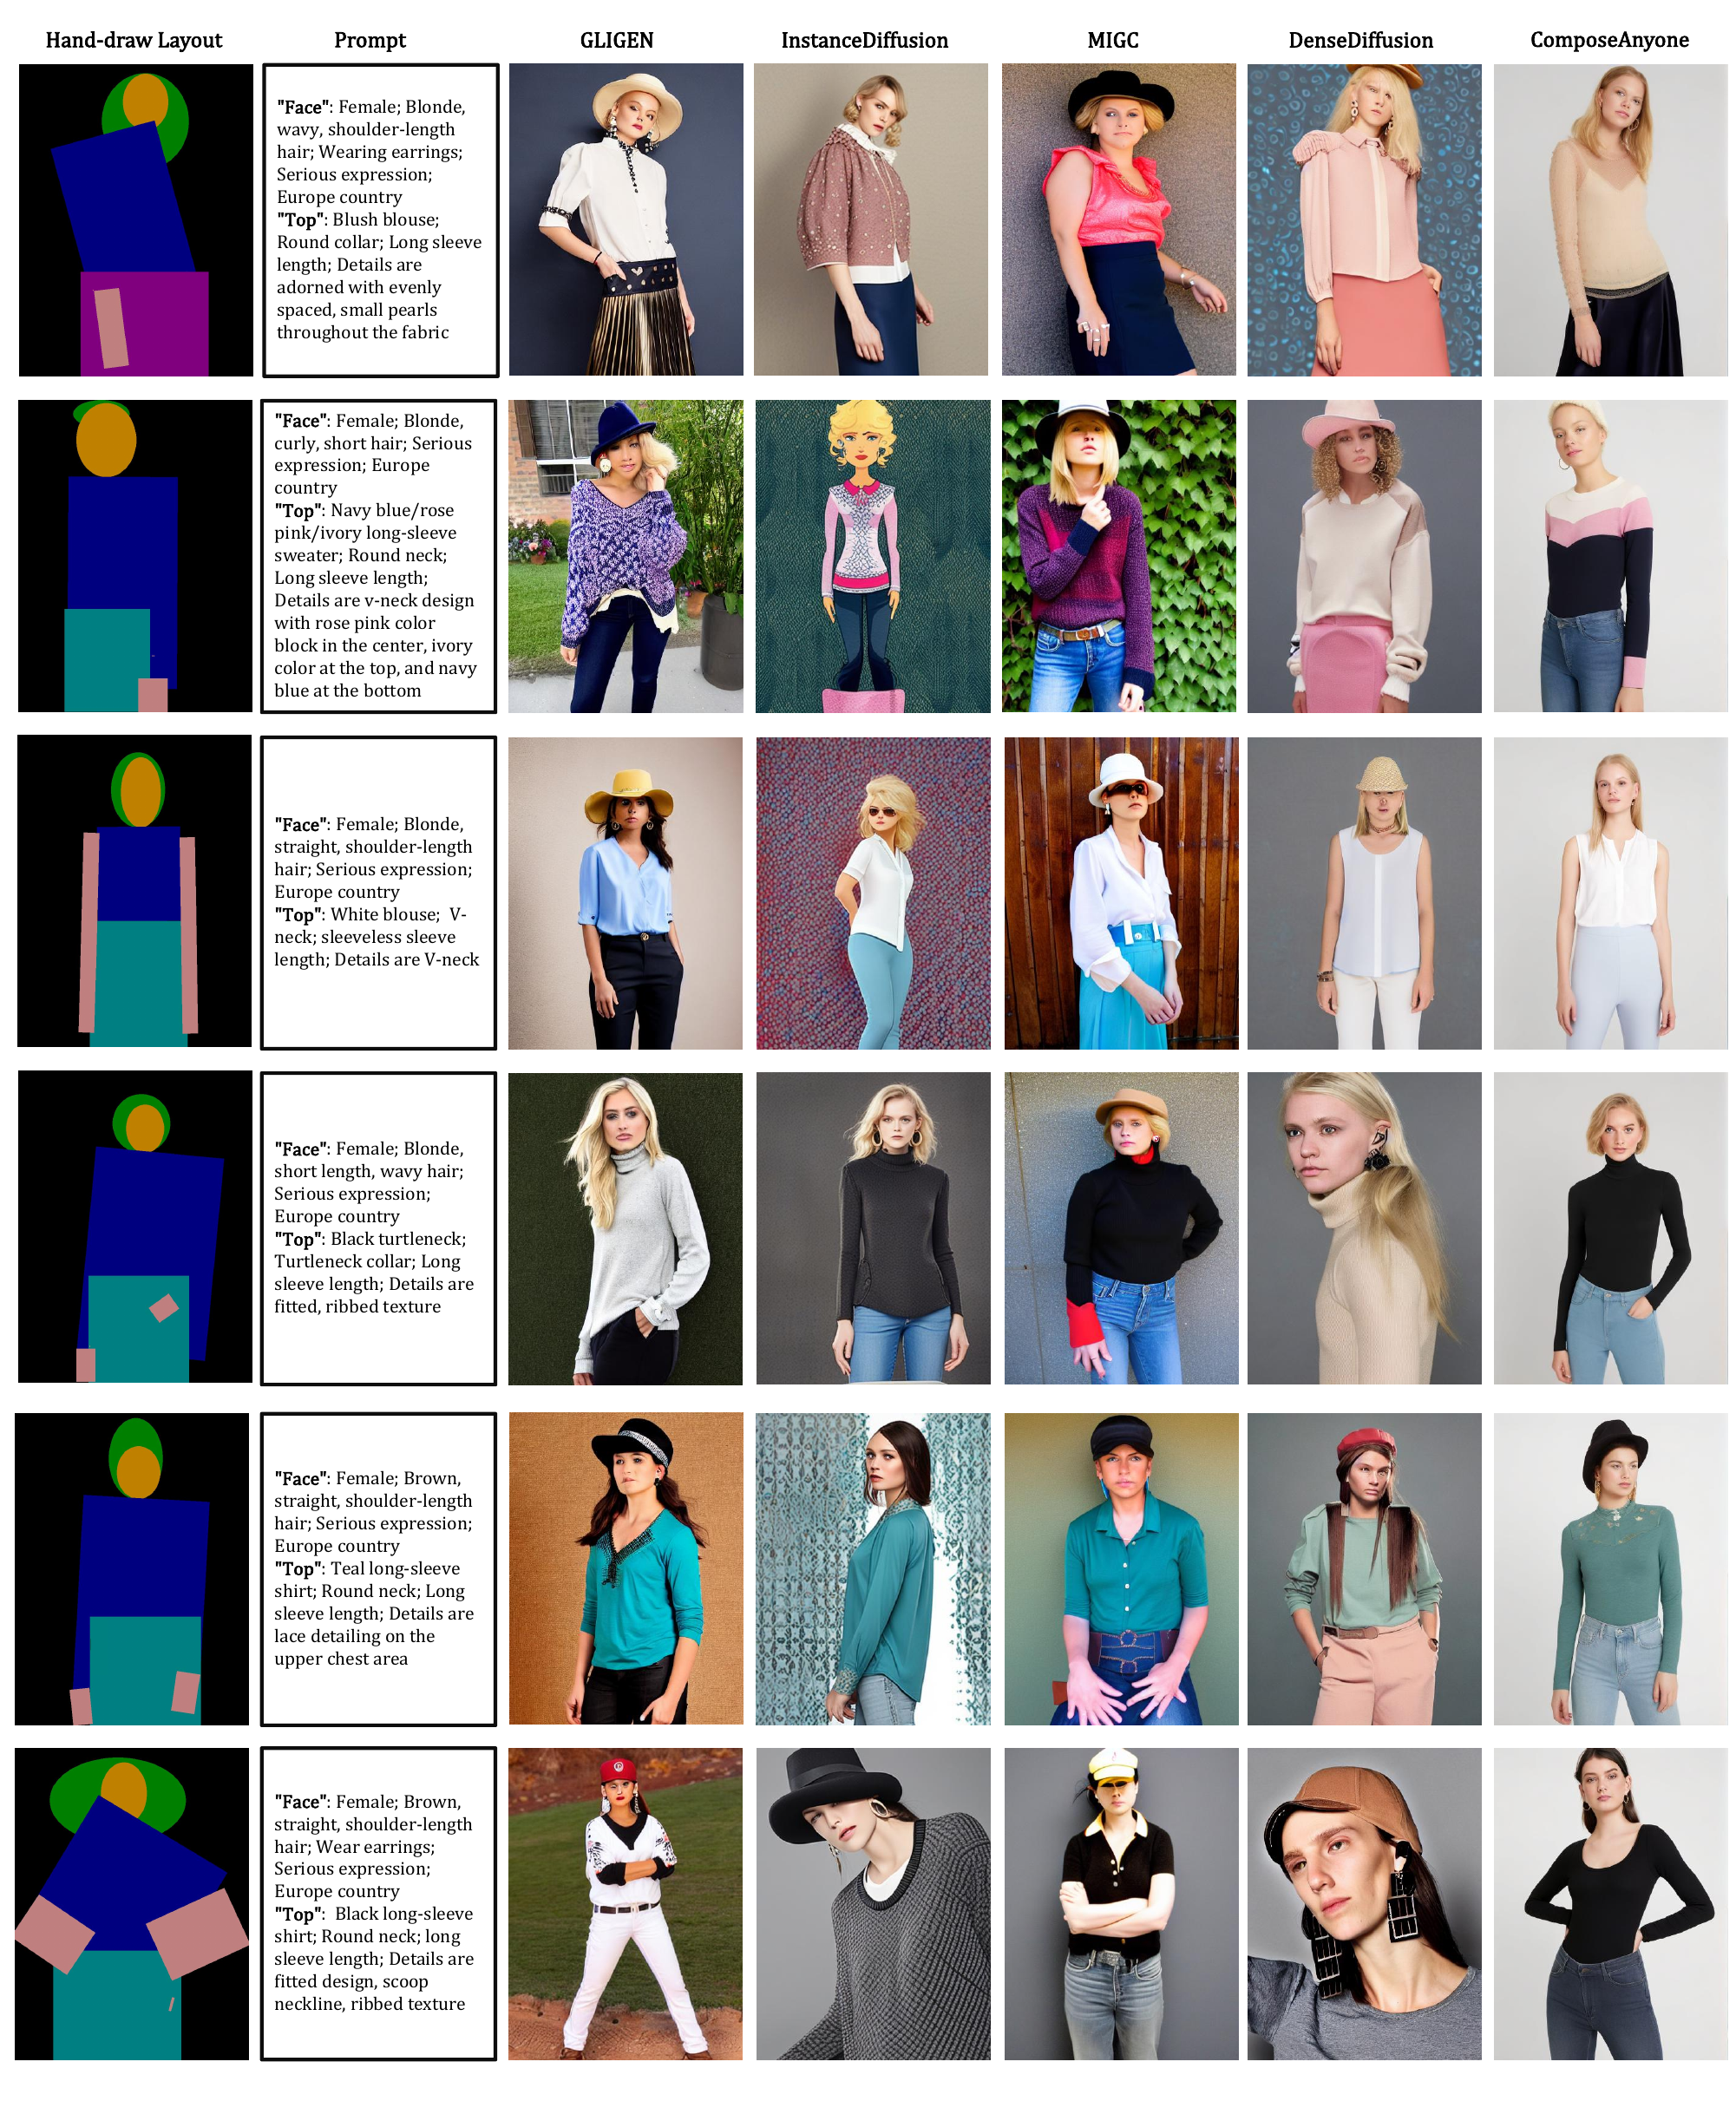}
  % \vspace{-2mm}
  \caption{More qualitative comparison with layout-guided text-to-image methods on the VITON-HD dataset. ComposeAnyone demonstrates a high level of congruity with both textual descriptions and spatial layout arrangements in its generative output.
  }
  % \vspace{-2mm}
  \label{fig:visual2}
\end{figure*}

% \section{Rationale}
% \label{sec:rationale}
% % 
% Having the supplementary compiled together with the main paper means that:
% % 
% \begin{itemize}
% \item The supplementary can back-reference sections of the main paper, for example, we can refer to \cref{sec:intro};
% \item The main paper can forward reference sub-sections within the supplementary explicitly (e.g. referring to a particular experiment); 
% \item When submitted to arXiv, the supplementary will already included at the end of the paper.
% \end{itemize}
% % 
% To split the supplementary pages from the main paper, you can use \href{https://support.apple.com/en-ca/guide/preview/prvw11793/mac#:~:text=Delete%20a%20page%20from%20a,or%20choose%20Edit%20%3E%20Delete).}{Preview (on macOS)}, \href{https://www.adobe.com/acrobat/how-to/delete-pages-from-pdf.html#:~:text=Choose%20%E2%80%9CTools%E2%80%9D%20%3E%20%E2%80%9COrganize,or%20pages%20from%20the%20file.}{Adobe Acrobat} (on all OSs), as well as \href{https://superuser.com/questions/517986/is-it-possible-to-delete-some-pages-of-a-pdf-document}{command line tools}.
